# Supplementary material for: Visual collective behaviors on spherical robots
Source: arXiv:2409.20539 source file (2025-01-16)
Supplement: Supplementary file 1 [file SuppData2.pdf]

# Supplementary information of Visual collective behaviors on spherical robots

**Diego Castro[1,2], Christophe Eloy[2] and Franck Ruffier[1,*]**

[1]Aix Marseille Université, CNRS, ISM, Marseille, 13288, France

[2]Aix Marseille Université, CNRS, Centrale Med, IRPHE, Marseille, 13013, France

[*]Author to whom any correspondence should be addressed.

E-mail: `franck.ruffier@cnrs.fr`

Submitted to: *Bioinspir. Biomim.*
16 January 2025

## S1 Spheros' dynamical response and time delay $\tau$ estimation

The robotic setup is composed of several steps, from setting a heading and velocity, to recognizing a XY-coordinate and heading from the image. Each step involves their own input treatment, response time and processing. As such, we performed a step response analysis for both heading and velocity independently. This analysis allows to see if there are what are significant changes from the intimidate response of the simulation.

Fig. S1 a, shows the average step response for a change in the heading of the robot. The change ranged from 1 to 180 degrees. Fig. S1 b, shows the average step response for a change in the velocity of the robot. The change ranged from 1 to 25 a/sec. Fig. S1 c, shows the average step response for a change in the yaw $\dot{\theta}$ of the robot. Fig. S1 d-e, shows this speeds ramps in the measured variables. All steps responses were performed 5 times with 10 different robots. The Y-axis is a percentage of the desired heading. Finally, Fig. S1 f, shows the measurement sensitivity to changes in heading and Fig. S1 g, shows the error in following a desired yaw $\dot{\theta}$. These results show that the system has a median time delay $\tau$ of approximately 600ms in responding to any input signal change. The image processing takes from 10-50ms, the image acquisition take from 25-50ms. Leaving at best 400ms delay to the communication between the control and the robot, the inner processing and the actuation of the input. Therefore, the visual input for the collective motion model must reflect this transport delay.

## S2 Direct comparison between Supplemented visual model and robot-in-the-loop Experiments

The difference between Phase Diagrams constructed from simulated and robots-in-the-loop experiments for 10 individuals is very marginal Fig. S2. The mean squared error

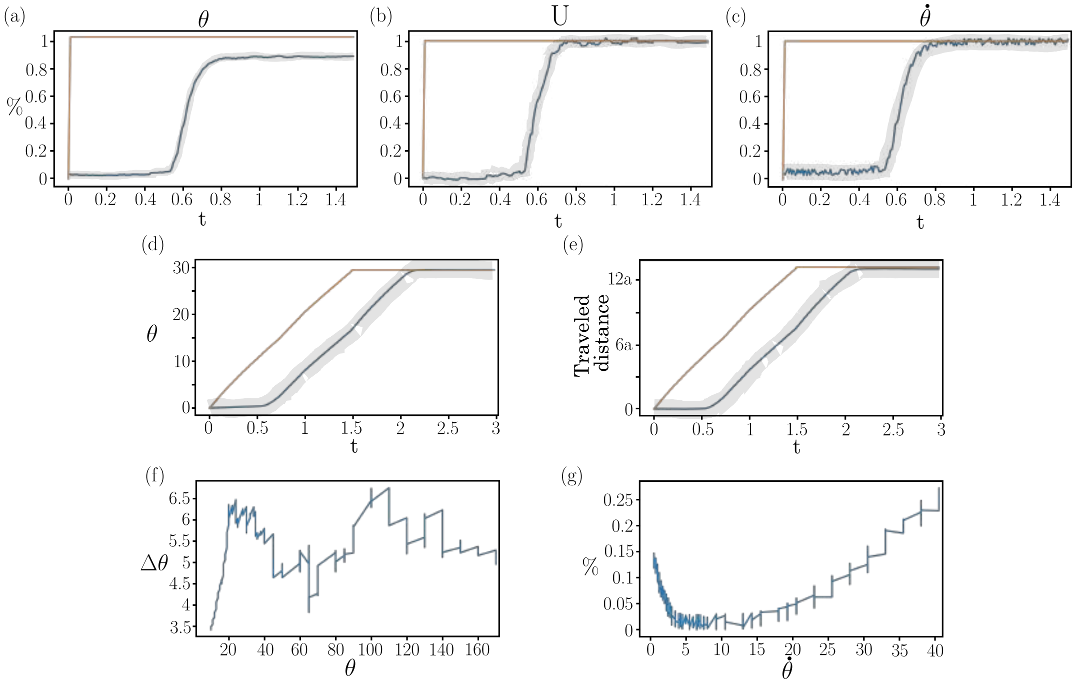


**Fig. S1.** Spheros' dynamical response (The grey shade is the average of normalized standard deviation) a) Average normalized heading $\theta$ step response of the 520 experiments. b) Average normalized velocity $U$ step response [a/sec] of the 220 experiments. c) Average normalized yaw $\dot{\theta}$ step response [degrees] of the 220 experiments. d) Average heading $\theta$ ramp response [degrees/sec] of the 220 experiments. e) Average velocity step response as seen in traveled distance (with $a = 3.5cm$) of the 220 experiments. f) Heading $\theta$ measurement average sensitivity in degrees of the 520 experiments. g) Yaw $\dot{\theta}$ measurement average sensitivity in percentage of the 520 experiments.

– MSE – between the phase diagram images of robots-in-the-loop and supplemented visual model is 2.48%.

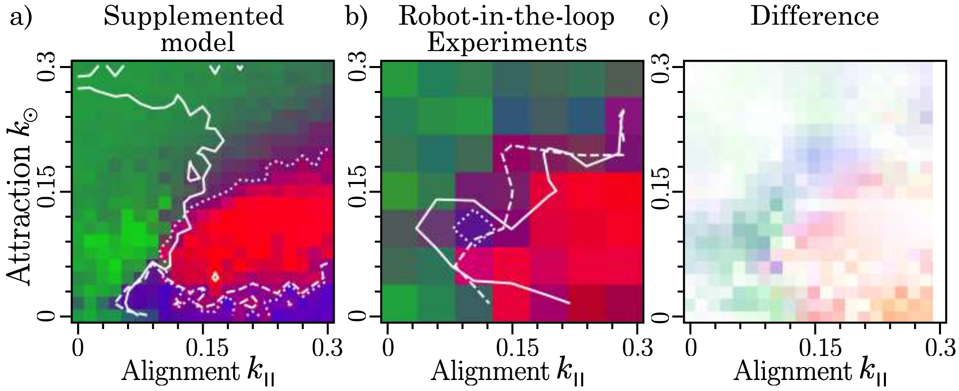


**Fig. S2.** Difference between the Phase Diagrams. a) Supplemented visual model (10 individuals), b) Phase Diagram of Spheros' robots-in-the-loop (10 robots), c) Raw difference image difference between both phase diagram. The mean squared error – MSE – between the phase diagram images of robots-in-the-loop and supplemented visual model is 2.48%.

## S3 Image Processing Technical information

The camera details are presented on Table S1 The detailed dual image segmentation

| | |
|---|---|
| Resolution | 1920x1200 |
| Frame rate | 168fps |
| Pixel Size | 5.86uM |
| Sensor Type | Sony IMX174 |
| Optical Size | 1/1.2” |
| Shutter Type | Global Shutter |
| Shutter time | 52us 1s |
| ADC Bit Depth | 10bit |
| Pixel Bit Depth | 8bit, 10bit |
| Digital gain | 0dB 24dB |
| Pixel Data Format | Bayer RG8 / Bayer RG10 |
| Lens mount | type-C |
| Power Consumption | ¡2.7W@5V |

**Table S1.** Camera: *Daheng Imaging MER2-230-168U3C* specifications.

example is presented on Fig. S3.

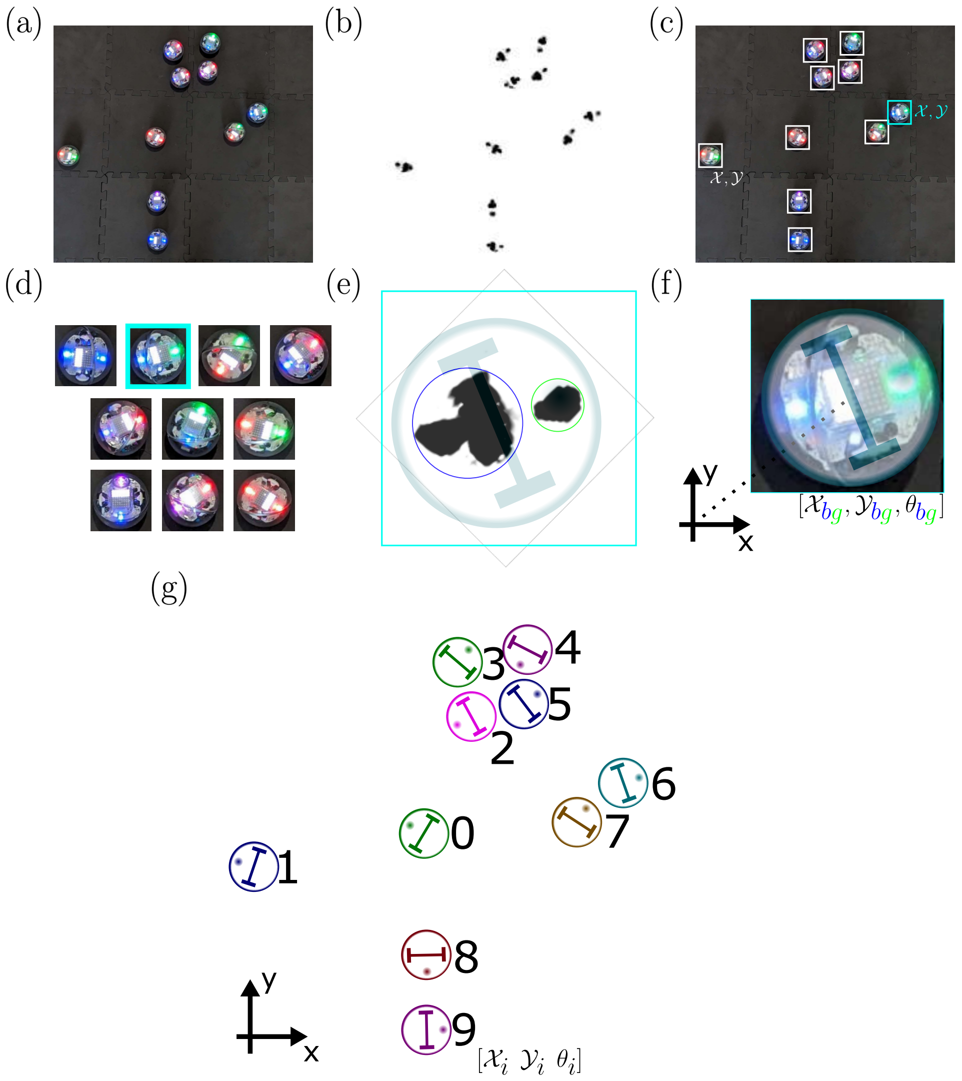


**Fig. S3.** Illustration of the phases observed for the original model. We observe three phases when varying the other two parameters: (a) Swarming ($k_{\odot} = 0.15$, $k_{\parallel} = 0$); (b) Schooling ($k_{\odot} = 0.07$, $k_{\parallel} = 0.3$); (c) Milling ($k_{\odot} = 0.07$, $k_{\parallel} = 0.05$).

*Feature Matching Optic Flow*

Fig. S4 showcases examples of what real world each of the components of the optic flow would look like. It also correlated each with a binary panorama equivalency. Finally it shows a mixed case that would be a normal optic flow generation for both image and 1D cases.

For the feature matching optic flow the gradient generated when the amount of retinal object differ between consecutive time steps is shown on Fig. S5.

## S4 Digital implementation of the supplemented visual model

The model presented on Eqs. 1, are the integral form of the model that use of the visual panorama. $\mathcal{V}_i(\phi, t-\tau)$ is a piece-wise constant function that can be expressed as a set unit boxcar functions (one for each retinal object).

Each retinal object can be described as a rising $\varphi_{\Uparrow k}$ and its corresponding falling edge $\varphi_{\Downarrow k}$. Furthermore, from these edges, we can compute the shade's mid-point $\varphi_k = (\varphi_{\Uparrow k} + \varphi_{\Downarrow k})/2$, and the retinal's object half-width $\Delta\varphi_k = (\varphi_{\Downarrow k} - \varphi_{\Uparrow k})/2$. The apparent distance, $\mathcal{R}_i(\phi, t-\tau)$ is defined as $\mathcal{V}_i(\phi, t-\tau)$ weighted by $\frac{a}{\sin \Delta\varphi_k}$, thus depending on the inverse of the optic size of the retinal object.

This means that $\mathcal{R}_i(\phi, t-\tau)$ for a binary $\mathcal{V}_i(\phi, t-\tau)$, is a function independent of $\phi$ and is only be dependent on the $k$-retinal's object half-width ($\mathcal{R}_k(\Delta\varphi_k)$). Similarly, the avoidance function can be expressed as a function of $\Delta\varphi_k$, and is independent of $\phi$. We add the subscript $k$, which identifies a single retinal object on the binary panorama of the individual $i$. Note that a retinal object $k$ is different from an individual $j$, as in a retinal object there can be occlusion or aggregation of any $j$-particles on the $i$-th binary panorama. Then, we can rewrite Eq. 1c as:

$$\omega_{\odot}(t) = \left\langle \sum_k \mathcal{R}_i^2(\Delta\varphi_k, t-\tau)\mathcal{A}(\Delta\varphi_k, t-\tau) \int_{\varphi_{\Uparrow k}}^{\varphi_{\Downarrow k}} b_\epsilon(\phi, t-\tau) \sin(\phi, t-\tau)\, d\phi. \right\rangle \tag{S1}$$

where $b_\epsilon(\phi, t-\tau) = 1 + \epsilon\cos(\phi, t-\tau)$. And developing the integral we get

$$\omega_{\odot}(t) = \langle \sum_k 2\mathcal{R}_i^2(\Delta\varphi_k, t-\tau)\mathcal{A}(\Delta\varphi_k, t-\tau) \sin(\Delta\varphi_k, t-\tau) \sin(\varphi_k, t-\tau) \\ (1 + \epsilon\cos(\varphi_k, t-\tau)\cos(\Delta\varphi_k, t-\tau))\rangle \tag{S2}$$

And here $\mathcal{R}_i(\Delta\varphi_k, t-\tau) = \frac{a}{\sin(\Delta\varphi_k, t-\tau)}$, Resulting in:

$$\omega_{\odot}(t) = \left\langle \sum_k \frac{2a^2\,(1 + \epsilon\cos(\varphi_k, t-\tau)\cos(\Delta\varphi_k, t-\tau))}{\sin(\Delta\varphi_k, t-\tau)} \sin(\varphi_k, t-\tau) \right\rangle \tag{S3}$$

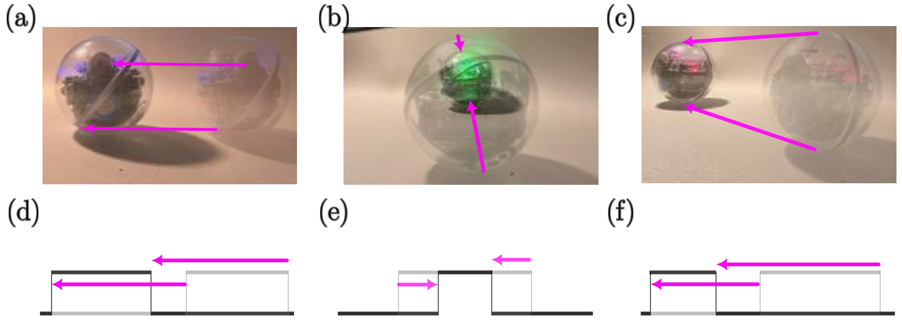


**Fig. S4.** Optic flow. a) Purely translational, b) Purely Convergent, c) Mixed Case, d) 1-D feature matching purely translational, d) 1-D feature matching purely convergent, d) 1-D feature matching mixed case.

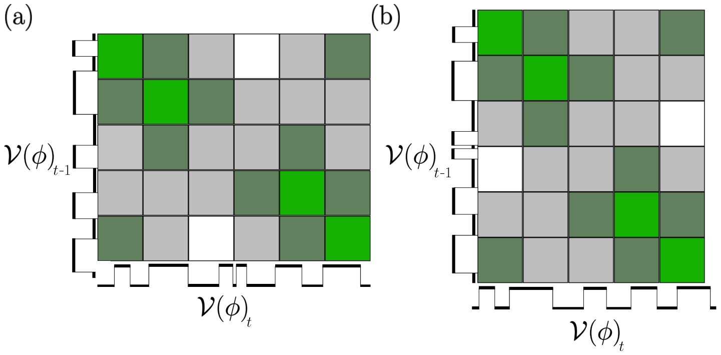


**Fig. S5.** Retinal object matching between consecutive time steps. a) Separation of retinal object, b) Merging of retinal objects.

By substituting the $\langle\cdot\rangle$ normalization the implemented equation is:

$$\omega_{\odot}(t) = \frac{\sum_k \frac{2a^2(1+\epsilon\cos(\varphi_k,t-\tau)\cos(\Delta\varphi_k,t-\tau))}{\sin(\Delta\varphi_k,t-\tau)}\sin(\varphi_k,t-\tau)}{\sum_k \frac{2a^2(1+\epsilon\cos(\varphi_k,t-\tau)\cos(\Delta\varphi_k,t-\tau))}{\sin(\Delta\varphi_k,t-\tau)}} \tag{S4}$$

The next step is to do the same for the alignment component. First, we replace Eq. 1f in Eq. 1d resulting in:

$$\omega_{\|}(t) = \int_{-\pi}^{\pi} U^{-1}(\overline{\mathcal{O}}_i(\phi,t-\tau)\cos(\phi,t-\tau) - \mathcal{D}_i(\phi,t-\tau)\sin(\phi,t-\tau))b_\epsilon(\phi,t-\tau)d\phi \tag{S5}$$

Note, that the visual alignment can also be written in polar coordinates $(\phi, r)$, with an azimuthal and radial component as follows:

$$\omega_{\|}(t) = \langle\omega_{\|,\phi}(t) + \omega_{\|,r}(t)\rangle \tag{S6}$$

$\mathcal{D}_i(\phi, t-\tau)$ and $\overline{\mathcal{O}}_i(\phi, t-\tau)$, similarly to $\mathcal{R}_i(\phi, t-\tau)$, are piece-wise constant function which are independent of $\phi$ but dependent on $\Delta\varphi_k$.

Taking Eq. S5 and Eq. S6:

$$\omega_{\|,\phi}(t) = \sum_k \mathcal{O}_i(\Delta\varphi_k,\phi,t-\tau)\left(\int_{\varphi_{\Uparrow k}}^{\varphi_{\Downarrow k}}\cos(\phi,t-\tau)b_\epsilon(\phi,t-\tau)d\phi\right) \tag{S7}$$

$$\omega_{\|,r}(t) = \sum_k -\mathcal{D}_i(\Delta\varphi_k,\phi,t-\tau)\left(\int_{\varphi_{\Uparrow k}}^{\varphi_{\Downarrow k}}\sin(\phi,t-\tau)b_\epsilon(\phi,t-\tau)d\phi\right) \tag{S8}$$

Eq. S8 is the exact form as Eq. S1 with the weight of the integral being $\mathcal{D}_i(\Delta\varphi_k, t-\tau)$ instead of $\mathcal{R}_i^2(\Delta\varphi_k, t-\tau)\mathcal{A}(\Delta\varphi_k, t-\tau)$ resulting in:

$$\omega_{\|,r}(t) = \sum_k \frac{-2\mathcal{D}_i(\Delta\varphi_k,t-\tau)}{\mathcal{R}_i(\Delta\varphi_k,t-\tau)}\sin(\varphi_k,t-\tau)\left(1+\epsilon\cos(\varphi_k,t-\tau)\cos(\Delta\varphi_k,t-\tau)\right) \tag{S9}$$

As for Eq. S7 the developing the integral and assuming $\Delta\phi \approx \sin\Delta\phi$ we have:

$$\begin{aligned}\omega_{\|,\phi}(t) = \sum_k \frac{\mathcal{O}_i(\Delta\varphi_k,t-\tau)}{\mathcal{R}_i(\Delta\varphi_k,t-\tau)}&(2\cos(\varphi_k,t-\tau)(1+\epsilon\cos(\Delta\varphi_k,t-\tau)\cos(\varphi_k,t-\tau))\\ &+\epsilon(1-\cos(\Delta\varphi_k,t-\tau)))\end{aligned} \tag{S10}$$

Assumming that $\cos\Delta\varphi_k \approx 1$ and using Eq. 1f, then Eqs. S9-S10 become:

$$\omega_{\|}(t) \approx \left\langle \sum_k 2\frac{\mathbf{e}_i(t-\tau)\times\mathbf{V}_{ik}(t-\tau)}{U\mathcal{R}_i^2(\Delta\varphi_k, t-\tau)} b_\epsilon(\varphi_k, t-\tau) \right\rangle \tag{S11}$$

Susbtituting the normalization and the blindspot, Eq. S11 becomes:

$$\omega_{\|}(t) \approx \frac{\sum_k 2\frac{\mathbf{e}_i(t-\tau)\times\mathbf{V}_{ik}(t-\tau)}{U\mathcal{R}_i^2(\Delta\varphi_k,t-\tau)}(1+\epsilon\cos(\varphi_k, t-\tau))}{\sum_k 2\frac{\|\mathbf{V}_{ik}(t-\tau)\|}{U\mathcal{R}_i^2(\Delta\varphi_k,t-\tau)}(1+\epsilon\cos(\varphi_k, t-\tau)} \tag{S12}$$

## S5 Original Visual Collective Motion Model (Castro *et al.*, 2024) [1]

Our model considers a system of $N$ self-propelled particles confined to a plane (Fig. 1a-b). Each particle is represented as an object with a radius $a$, moving with a constant speed $U$. The position of each particle is denoted by $\mathbf{x}_i$, and its orientation is described by the unit vector $\mathbf{e}_i = [\cos\theta_i, \sin\theta_i]$. The collective motion model interacts with the particles by adjusting their angular velocity at each time step.

$$\dot{\mathbf{x}}_i = U\mathbf{e}_i, \tag{S13}$$

$$\dot{\theta}_i = k_\odot\,\omega_\odot + k_\|\,\omega_\| + k_\eta\,\eta, \tag{S14}$$

We represent the visual surroundings of the particles as retinal objects on a one-dimensional (1-D) binary panorama (Fig. 1c). This binary panorama is centered on the focal particle's heading, marking the presence of objects along the line of sight and generating binary retinal objects (Fig. 1d). Since all particles are perceived with the same magnitude, multiple particles may aggregate into a single, larger retinal object. Consequently, there are typically more $i$-particles than $k$-retinal objects. A apparent distance ($\mathcal{R}_i(\phi)$) is computed from this binary panorama (Fig. 1e), which is then used to calculate the attraction component of the angular velocity, $\omega_\odot$ (Eq. S15).

The optic flow perceived by each particle (illustrated by the black arrows in Fig. 1c) can be decomposed into two components: a radial component representing the translational optic flow (the average of the function shown in Fig. 1f), and an azimuthal component representing the divergence or convergence of the optic flow (Fig. 1g). The apparent velocity vector for each retinal object ($V_{i,k}$) can be determined using these two components of optic flow. This apparent velocity is employed to compute the alignment component of the angular velocity, $\omega_\|$ (Eq. S16). Finally, the individuality of each particle is incorporated into the angular velocity as a standard Wiener process ($\eta$).

$$\omega_\odot = \left\langle \int_{-\pi}^{\pi} \mathcal{R}_i^2(\phi) b_\epsilon(\phi)\sin\phi\, d\phi \right\rangle, \tag{S15}$$

$$\omega_\| = \left\langle \int_{-\pi}^{\pi} \frac{\mathbf{e}_i\times\mathbf{V}_{ik}}{U\mathcal{R}_i(\phi)} b_\epsilon(\phi)\, d\phi \right\rangle, \tag{S16}$$

$$\frac{\mathbf{e}_i\times\mathbf{V}_{ik}}{U\mathcal{R}_i(\phi)} = \frac{-\mathcal{D}_i(\phi)\sin\phi + \overline{\mathcal{O}}_i(\phi)\cos\phi}{U}. \tag{S17}$$

$b_\epsilon(\phi)$ is a parametric representation of an optic blind spot. The operand $\langle\cdot\rangle$ denotes a normalization that ensures the resulting function is of order $O(1)$. Conceptually, it functions like a min-max normalization on the amount of rotation for a single time step.

This model is made dimensionless by using $a$ as the spatial unit and $a/U$ as the temporal unit. The use of these spatial and temporal units creates a parameter space with the weights of each component of the angular velocity $(k_\odot, k_\parallel, k_\eta)$. Some Results can be seen on Fig. S6.

## S6 Observed phases

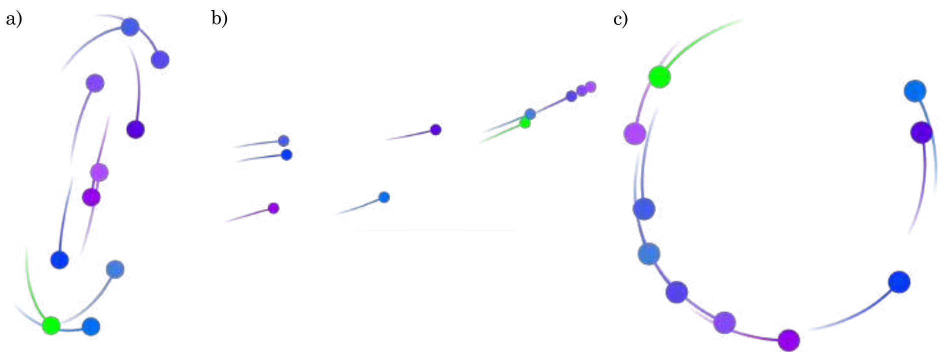


**Fig. S6.** Illustration of the phases observed for the raw original model [1]. We observe three phases when varying the other two parameters: (a) Swarming ($k_\odot = 0.15$, $k_\parallel = 0$) (see Svideo 13); (b) Schooling ($k_\odot = 0.07$, $k_\parallel = 0.3$) (see Svideo 14); (c) Milling ($k_\odot = 0.07$, $k_\parallel = 0.05$) (see Svideo 15).

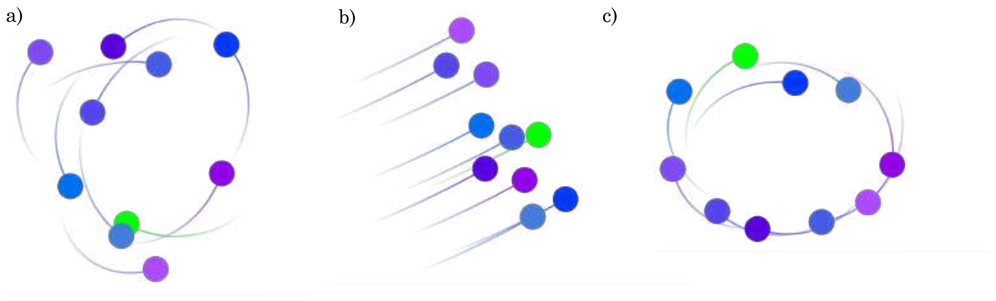


**Fig. S7.** Illustration of the phases observed for the visual model supplemented only with the avoidance. We observe three phases when varying the other two parameters: (a) Swarming ($k_\odot = 0.07$, $k_\parallel = 0$) (see Svideo 16); (b) Schooling ($k_\odot = 0.15$, $k_\parallel = 0.3$) (see Svideo 17); (c) Milling ($k_\odot = 0.07$, $k_\parallel = 0.05$) (see Svideo 18).

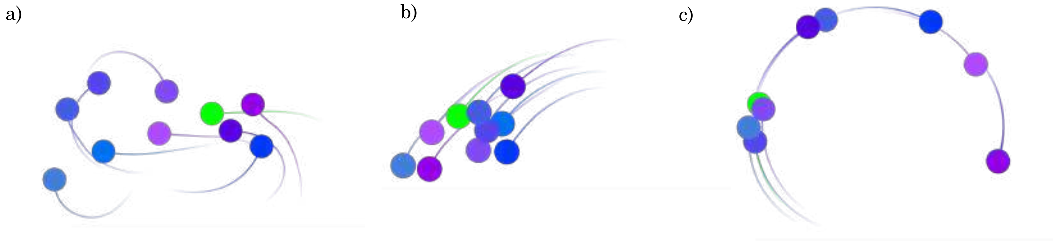


**Fig. S8.** Illustration of the phases observed for the visual model supplemented only with the avoidance and the visual anchor. We observe three phases when varying the other two parameters: (a) Swarming ($k_{\odot} = 0.3$, $k_{\parallel} = 0$) (see Svideo 19); (b) Schooling ($k_{\odot} = 0$, $k_{\parallel} = 0.3$) (see Svideo 20); (c) Milling ($k_{\odot} = 0.07$, $k_{\parallel} = 0.3$) (see Svideo 21).

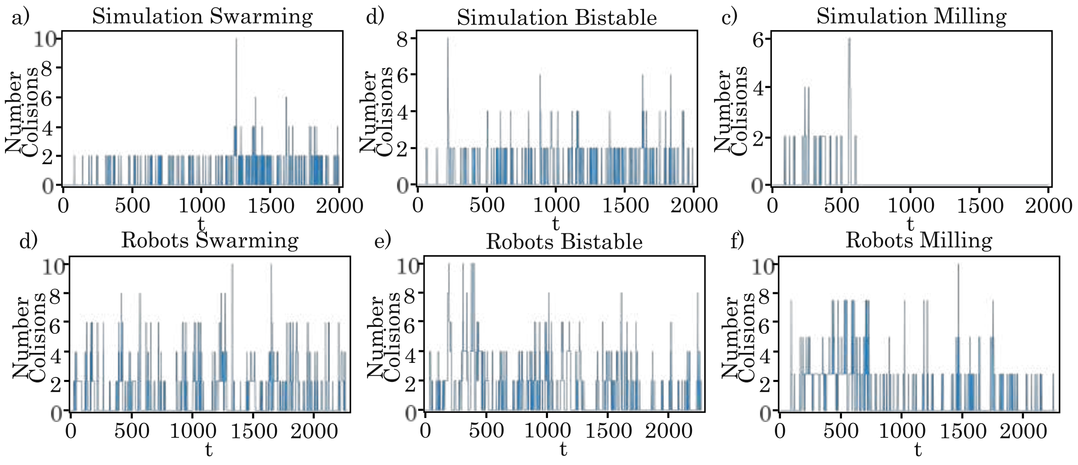


**Fig. S9.** Number of collisions during the evolution with a set of parameters (a) Swarming simulation; (b) Schooling simulation; (c) Milling simulation; (d) Swarming robot-in-the-loop; (e) Schooling robot-in-the-loop; (f) Milling robot-in-the-loop.

## S7 Occlusion Analysis

## References

[1] Castro D, Ruffier F and Eloy C 2024 *Phys. Rev. Res.* **6**(2) 023016 URL `https://link.aps.org/doi/10.1103/PhysRevResearch.6.023016`

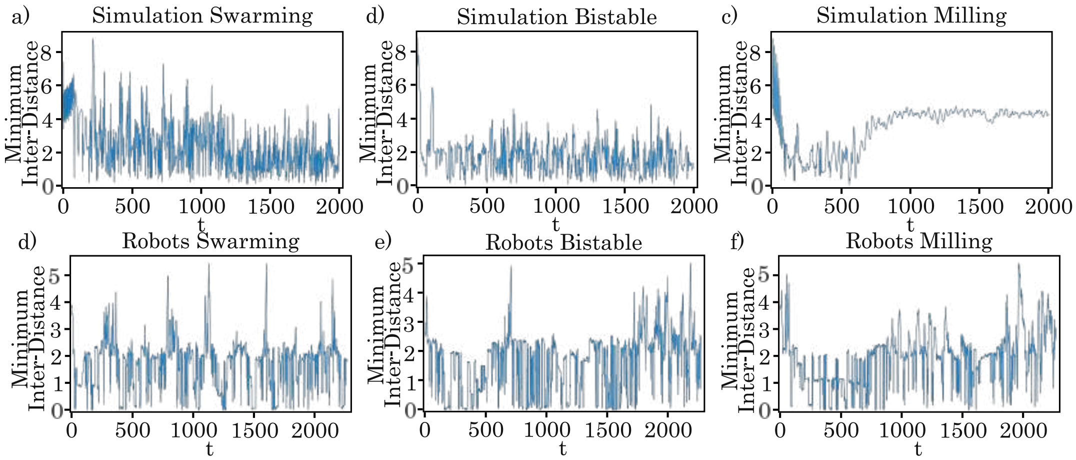


**Fig. S 10.** Minimum inter-distance found during the evolution with a set of parameters (a) Swarming simulation; (b) Schooling simulation; (c) Milling simulation; (d) Swarming robot-in-the-loop; (e) Schooling robot-in-the-loop; (f) Milling robot-in-the-loop.
